# Supplementary material for: Architectures of Meaning, A Systematic Corpus Analysis of NLP Systems
Source: arXiv:2107.08124 ancillary file (2021-07-16)
Supplement: Supplementary file 1 [file arxiv_Architectures_of_meaning_Appendix.pdf]

# Architectures of Meaning: A Systematic Corpus Analysis of NLP Systems
# Appendix

Lexicon of Section Headings:

Headings containing words *introduction*, *related*, *previous*, *background*, *literature*, *of the art*, and words: *results*, conclusions were associated with sections considered as the *opening* and the *end* of the paper, respectively. As both of them are likely to mention previous works/systems, only the sections between *opening* and end were processed further (note: as a result the *title*, abstract and *references* were removed as well).

Pre-processing Heuristics:

Blocks were merged into one block of text (one per paper) and pre-processed using the filters: removed sentences containing a word *baseline*, removed punctuation, lower cased, removed double spaces and line breaks. In each text the algorithm searches for an exact string match with an entity in the lexicon.

To each entity string white spaces from both sides were added ('lstm' to ' lstm '), in order to eliminate substrings detection (e.g. 'lstm' in 'bilstm'). Each entity was also checked in the plural.

Automatic Extraction:

Using our algorithm we were able to extract text from 96.3\% of the target papers (1039 out of 1079). In 40 cases the text was extracted manually. Although sections like Introduction, *Related Work*, *Results* and *Conclusions* were excluded from the search, detection of baselines or models developed in previous studies/years is possible. One obvious reason is that the key section with description of a newly proposed model contains comparison to previous models. Another reason is the possibility of finding ’related work’ sections both at the beginning and at the end of the paper, as the sections order in the paper is not strictly imposed. Finally, components are taken out of context and negations are counted equally to the true usage.

## 1. Top 100 Components from SemEval 2019

| No | Component | Coefficient | R2 |
|---|---|---|---|
| 1 | LSTM | 0.147 | 0.95 |
| 2 | Word Embeddings | 0.125 | 0.911 |

| | | | |
|---|---|---|---|
| 3 | embedding layer | 0.108 | 0.969 |
| 4 | BiLSTM | 0.093 | 0.922 |
| 5 | fastText | 0.092 | 1 |
| 6 | softmax | 0.088 | 0.971 |
| 7 | GloVe | 0.087 | 0.991 |
| 8 | attention layer | 0.073 | 0.874 |
| 9 | adam | 0.067 | 0.988 |
| 10 | RNN | 0.061 | 0.839 |
| 11 | dense layer | 0.061 | 0.885 |
| 12 | CNN | 0.054 | 0.889 |
| 13 | w2v | 0.048 | 0.352 |
| 14 | encoder | 0.047 | 0.897 |
| 15 | fully connected layer | 0.042 | 0.888 |
| 16 | FNN | 0.041 | 0.74 |
| 17 | pooling | 0.031 | 0.81 |
| 18 | PyTorch | 0.031 | 1 |
| 19 | transformer | 0.028 | 0.523 |
| 20 | logistic regression | 0.028 | 0.86 |
| 21 | scikit-learn | 0.025 | 0.921 |
| 22 | lower case | 0.024 | 0.657 |
| 23 | RF | 0.023 | 0.664 |
| 24 | GRU | 0.021 | 0.913 |
| 25 | Tensorflow | 0.021 | 0.793 |
| 26 | ensemble model | 0.02 | 0.734 |
| 27 | term frequency | 0.02 | 0.673 |
| 28 | Deep Learning | 0.017 | 0.781 |
| 29 | NLTK | 0.016 | 0.699 |
| 30 | IDF | 0.015 | 0.446 |
| 31 | MLP | 0.015 | 0.759 |
| 32 | DNN | 0.013 | 0.589 |
| 33 | tokenization | 0.012 | 0.252 |
| 34 | CLSTM | 0.012 | 1 |
| 35 | skipgram | 0.01 | 0.114 |
| 36 | fully connected layers | 0.008 | 0.05 |
| 37 | character embedding | 0.008 | 0.704 |
| 38 | decoder | 0.007 | 0.905 |
| 39 | SVM | 0.006 | 0.024 |
| 40 | GBM | 0.006 | 0.517 |
| 41 | character n-grams | 0.006 | 0.238 |
| 42 | attention model | 0.005 | 0.088 |

| | | | |
|---|---|---|---|
| 43 | Scikit learn | 0.005 | 0.758 |
| 44 | CoreNLP | 0.004 | 0.082 |
| 45 | BiRNN | 0.004 | 0.562 |
| 46 | KNN | 0.003 | 0.108 |
| 47 | layer normalization | 0.003 | 1 |
| 48 | DL | 0.003 | 0.187 |
| 49 | adaboost | 0.002 | 0.042 |
| 50 | linguistic features | 0.002 | 0.062 |
| 51 | bagging | 0.001 | 0.009 |
| 52 | bag of n-grams | 0 | 0.023 |
| 53 | AllenNLP | 0 | -inf |
| 54 | OpenAI | 0 | |
| 55 | fuzzy clustering | 0 | -inf |
| 56 | ELMo | 0 | |
| 57 | BERT | 0 | -inf |
| 58 | genetic algorithm | 0 | 0 |
| 59 | Autoencoder | 0 | 0 |
| 60 | LDA | 0 | 0.002 |
| 61 | deleted punctuation | -0.001 | 0.026 |
| 62 | decision tree | -0.001 | 0.003 |
| 63 | word2phrase | -0.001 | 0.786 |
| 64 | DAN | -0.001 | 1 |
| 65 | boosting algorithm | -0.001 | 0.27 |
| 66 | chi-square | -0.001 | 0.285 |
| 67 | Depth-first Search | -0.001 | 0.704 |
| 68 | GNN | -0.002 | 0.674 |
| 69 | BoW | -0.002 | 0.018 |
| 70 | IG | -0.002 | 0.687 |
| 71 | BoC | -0.002 | 0.674 |
| 72 | k-means | -0.003 | 0.256 |
| 73 | feature selection | -0.003 | 0.108 |
| 74 | constituency parser | -0.003 | 0.42 |
| 75 | Bayesian Network | -0.004 | 0.533 |
| 76 | ME | -0.004 | 0.651 |
| 77 | Breadth-first Search | -0.004 | 0.448 |
| 78 | CBOW | -0.004 | 0.023 |
| 79 | Brown | -0.005 | 0.054 |
| 80 | word clusters | -0.005 | 0.122 |
| 81 | rule based | -0.005 | 0.146 |
| 82 | clustering | -0.005 | 0.039 |

| | | | |
|---|---|---|---|
| 83 | steeming | -0.006 | 0.316 |
| 84 | classification | -0.008 | 0.312 |
| 85 | linear regression | -0.008 | 0.187 |
| 86 | stopword removal | -0.008 | 0.111 |
| 87 | Bayes classifier | -0.009 | 0.127 |
| 88 | n-grams | -0.01 | 0.049 |
| 89 | lexical features | -0.01 | 0.035 |
| 90 | PCA | -0.011 | 0.435 |
| 91 | NER | -0.013 | 0.234 |
| 92 | syntactic features | -0.014 | 0.652 |
| 93 | normalization | -0.017 | 0.43 |
| 94 | heuristic | -0.017 | 0.857 |
| 95 | dependency parsing | -0.031 | 0.658 |
| 96 | disambiguation | -0.035 | 0.894 |
| 97 | alignment | -0.036 | 0.572 |
| 98 | semantic features | -0.042 | 0.445 |
| 99 | lemmatization | -0.043 | 0.889 |
| 100 | POS tagging | -0.048 | 0.459 |

## 2. List of Top 100 Collocations from SemEval 2019

| Rank | Collocation | $freq_A$ | $freq_B$ | $freq_{AB}$ | $freq_{ABexp}$ | $\frac{freq_{AB}}{total\ \#\ of\ collocations}$ | $PMI$ | $t$ | $G^2$ | α |
|---|---|---|---|---|---|---|---|---|---|---|
| 1 | IDF & term frequency | 707 | 754 | 47 | 15.0 | 0.0013 | 1.64 | 3.04 | 46.09 | 3.43 |
| 2 | BERT & transformer | 506 | 400 | 27 | 5.7 | 0.0008 | 2.24 | 3.15 | 43.40 | 5.22 |
| 3 | CNN & pooling | 983 | 684 | 40 | 19.0 | 0.0011 | 1.08 | 2.27 | 18.75 | 2.23 |
| 4 | SVM & term frequency | 935 | 754 | 41 | 19.9 | 0.0012 | 1.04 | 2.24 | 18.19 | 2.17 |
| 5 | clustering & k-means | 114 | 61 | 4 | 0.2 | 0.0001 | 4.35 | 3.10 | 16.88 | 22.49 |
| 6 | BiLSTM & LSTM | 819 | 1428 | 58 | 33.0 | 0.0016 | 0.81 | 2.12 | 16.67 | 1.85 |
| 7 | BERT & encoder | 506 | 573 | 22 | 8.2 | 0.0006 | 1.43 | 2.27 | 16.61 | 2.84 |
| 8 | encoder & transformer | 573 | 400 | 19 | 6.5 | 0.0005 | 1.55 | 2.30 | 16.57 | 3.10 |
| 9 | IDF & SVM | 707 | 935 | 38 | 18.7 | 0.0011 | 1.03 | 2.16 | 16.35 | 2.14 |
| 10 | SVM & scikit-learn | 935 | 490 | 29 | 12.9 | 0.0008 | 1.17 | 2.16 | 15.54 | 2.36 |
| 11 | character n-grams & n-grams | 341 | 1046 | 24 | 10.1 | 0.0007 | 1.25 | 2.13 | 14.62 | 2.52 |
| 12 | character n-grams & skipgram | 341 | 272 | 10 | 2.6 | 0.0003 | 1.93 | 2.19 | 12.41 | 4.02 |
| 13 | POS tagging & lexical features | 636 | 548 | 22 | 9.8 | 0.0006 | 1.16 | 1.96 | 11.61 | 2.33 |
| 14 | BiRNN & character embedding | 66 | 101 | 3 | 0.2 | 0.0001 | 4.00 | 2.70 | 11.19 | 17.14 |
| 15 | steeming & stopword removal | 352 | 814 | 19 | 8.1 | 0.0005 | 1.23 | 1.94 | 11.13 | 2.46 |
| 16 | PyTorch & transformer | 169 | 400 | 8 | 1.9 | 0.0002 | 2.07 | 2.14 | 11.07 | 4.42 |
| 17 | SVM & n-grams | 935 | 1046 | 46 | 27.6 | 0.0013 | 0.74 | 1.81 | 10.91 | 1.73 |
| 18 | Bayes classifier & SVM | 289 | 935 | 18 | 7.6 | 0.0005 | 1.24 | 1.91 | 10.67 | 2.48 |
| 19 | lemmatization & stopword removal | 447 | 814 | 22 | 10.3 | 0.0006 | 1.10 | 1.87 | 10.55 | 2.23 |
| 20 | fully connected layer & pooling | 551 | 684 | 22 | 10.6 | 0.0006 | 1.05 | 1.80 | 9.69 | 2.15 |
| 21 | POS tagging & dependency parsing | 636 | 96 | 7 | 1.7 | 0.0002 | 2.02 | 2.01 | 9.42 | 4.34 |
| 22 | RF & SVM | 412 | 935 | 22 | 10.9 | 0.0006 | 1.02 | 1.75 | 9.21 | 2.11 |
| 23 | Bayes classifier & logistic regression | 289 | 771 | 15 | 6.3 | 0.0004 | 1.25 | 1.80 | 9.03 | 2.49 |
| 24 | lemmatization & linear regression | 447 | 184 | 8 | 2.3 | 0.0002 | 1.78 | 1.90 | 8.69 | 3.60 |
| 25 | LSTM & softmax | 1428 | 1175 | 68 | 47.4 | 0.0019 | 0.52 | 1.58 | 8.62 | 1.49 |
| 26 | linear regression & logistic regression | 184 | 771 | 11 | 4.0 | 0.0003 | 1.46 | 1.81 | 8.58 | 2.89 |
| 27 | NER & dependency parsing | 227 | 96 | 4 | 0.6 | 0.0001 | 2.70 | 2.11 | 8.38 | 6.85 |
| 28 | GRU & character embedding | 349 | 101 | 5 | 1.0 | 0.0001 | 2.33 | 2.01 | 8.34 | 5.30 |
| 29 | BERT & PyTorch | 506 | 169 | 8 | 2.4 | 0.0002 | 1.73 | 1.85 | 8.25 | 3.47 |
| 30 | SVM & logistic regression | 935 | 771 | 34 | 20.3 | 0.0010 | 0.74 | 1.60 | 8.07 | 1.73 |
| 31 | BiRNN & GRU | 66 | 349 | 4 | 0.7 | 0.0001 | 2.62 | 2.05 | 8.04 | 6.55 |
| 32 | IG & feature selection | 59 | 204 | 3 | 0.3 | 0.0001 | 3.14 | 2.19 | 7.91 | 9.37 |
| 33 | decoder & encoder | 123 | 573 | 7 | 2.0 | 0.0002 | 1.82 | 1.83 | 7.85 | 3.70 |
| 34 | RNN & character embedding | 711 | 101 | 7 | 2.0 | 0.0002 | 1.79 | 1.80 | 7.70 | 3.66 |
| 35 | FNN & fully connected layers | 451 | 199 | 8 | 2.5 | 0.0002 | 1.66 | 1.78 | 7.69 | 3.29 |
| 36 | LSTM & embedding layer | 1428 | 973 | 57 | 39.2 | 0.0016 | 0.54 | 1.51 | 7.64 | 1.50 |
| 37 | Bayes classifier & term frequency | 289 | 754 | 14 | 6.2 | 0.0004 | 1.19 | 1.66 | 7.64 | 2.37 |
| 38 | LSTM & RNN | 1428 | 711 | 44 | 28.7 | 0.0012 | 0.62 | 1.52 | 7.57 | 1.59 |
| 39 | FNN & rule based | 451 | 123 | 6 | 1.6 | 0.0002 | 1.94 | 1.83 | 7.46 | 4.02 |
| 40 | BiLSTM & softmax | 819 | 1175 | 42 | 27.2 | 0.0012 | 0.63 | 1.51 | 7.42 | 1.60 |
| 41 | AllenNLP & ELMo | 53 | 480 | 4 | 0.7 | 0.0001 | 2.48 | 1.95 | 7.41 | 5.99 |
| 42 | RF & logistic regression | 412 | 771 | 18 | 9.0 | 0.0005 | 1.01 | 1.59 | 7.34 | 2.08 |
| 43 | lexical features & syntactic features | 548 | 104 | 6 | 1.6 | 0.0002 | 1.90 | 1.79 | 7.24 | 3.93 |
| 44 | scikit-learn & term frequency | 490 | 754 | 20 | 10.4 | 0.0006 | 0.94 | 1.57 | 7.22 | 1.98 |
| 45 | attention layer & encoder | 646 | 573 | 20 | 10.4 | 0.0006 | 0.94 | 1.56 | 7.18 | 1.98 |

| | | | | | | | | | | |
|---|---|---|---|---|---|---|---|---|---|---|
| 46 | GRU & RNN | 349 | 711 | 15 | 7.0 | 0.0004 | 1.10 | 1.60 | 7.14 | 2.22 |
| 47 | BiLSTM & attention layer | 819 | 646 | 26 | 14.9 | 0.0007 | 0.80 | 1.52 | 7.05 | 1.80 |
| 48 | LSTM & attention layer | 1428 | 646 | 40 | 26.0 | 0.0011 | 0.62 | 1.45 | 6.89 | 1.59 |
| 49 | POS tagging & linguistic features | 636 | 184 | 9 | 3.3 | 0.0003 | 1.45 | 1.65 | 6.88 | 2.84 |
| 50 | OpenAI & transformer | 70 | 400 | 4 | 0.8 | 0.0001 | 2.34 | 1.85 | 6.73 | 5.35 |
| 51 | LSTM & Word Embeddings | 1428 | 2076 | 107 | 83.7 | 0.0030 | 0.35 | 1.35 | 6.67 | 1.32 |
| 52 | attention layer & decoder | 646 | 123 | 7 | 2.2 | 0.0002 | 1.64 | 1.67 | 6.65 | 3.27 |
| 53 | Bayes classifier & RF | 289 | 412 | 9 | 3.4 | 0.0003 | 1.42 | 1.62 | 6.64 | 2.77 |
| 54 | n-grams & term frequency | 1046 | 754 | 35 | 22.3 | 0.0010 | 0.65 | 1.43 | 6.59 | 1.62 |
| 55 | BoW & stopword removal | 470 | 814 | 20 | 10.8 | 0.0006 | 0.89 | 1.49 | 6.54 | 1.91 |
| 56 | feature selection & stopword removal | 204 | 814 | 11 | 4.7 | 0.0003 | 1.23 | 1.54 | 6.40 | 2.44 |
| 57 | BiLSTM & adam | 819 | 699 | 27 | 16.2 | 0.0008 | 0.74 | 1.43 | 6.36 | 1.72 |
| 58 | lexical features & n-grams | 548 | 1046 | 27 | 16.2 | 0.0008 | 0.74 | 1.43 | 6.35 | 1.72 |
| 59 | BiRNN & RNN | 66 | 711 | 5 | 1.3 | 0.0001 | 1.92 | 1.68 | 6.17 | 4.02 |
| 60 | CNN & softmax | 983 | 1175 | 47 | 32.6 | 0.0013 | 0.53 | 1.33 | 6.00 | 1.48 |
| 61 | FNN & softmax | 451 | 1175 | 25 | 15.0 | 0.0007 | 0.74 | 1.38 | 5.92 | 1.73 |
| 62 | dense layer & embedding layer | 778 | 973 | 33 | 21.4 | 0.0009 | 0.63 | 1.33 | 5.75 | 1.59 |
| 63 | decoder & transformer | 123 | 400 | 5 | 1.4 | 0.0001 | 1.85 | 1.62 | 5.73 | 3.75 |
| 64 | embedding layer & softmax | 973 | 1175 | 46 | 32.3 | 0.0013 | 0.51 | 1.27 | 5.53 | 1.46 |
| 65 | n-grams & scikit-learn | 1046 | 490 | 24 | 14.5 | 0.0007 | 0.73 | 1.33 | 5.52 | 1.71 |
| 66 | ELMo & encoder | 480 | 573 | 15 | 7.8 | 0.0004 | 0.95 | 1.38 | 5.49 | 1.99 |
| 67 | clustering & lemmatization | 114 | 447 | 5 | 1.4 | 0.0001 | 1.80 | 1.57 | 5.48 | 3.62 |
| 68 | linguistic features & syntactic features | 184 | 104 | 3 | 0.5 | 0.0001 | 2.47 | 1.74 | 5.46 | 5.77 |
| 69 | RNN & attention layer | 711 | 646 | 22 | 13.0 | 0.0006 | 0.76 | 1.33 | 5.45 | 1.74 |
| 70 | IDF & n-grams | 707 | 1046 | 32 | 20.9 | 0.0009 | 0.62 | 1.28 | 5.40 | 1.58 |
| 71 | FNN & Scikit learn | 451 | 115 | 5 | 1.5 | 0.0001 | 1.77 | 1.55 | 5.35 | 3.55 |
| 72 | Bayes classifier & IDF | 289 | 707 | 12 | 5.8 | 0.0003 | 1.06 | 1.38 | 5.32 | 2.15 |
| 73 | NLTK & stopword removal | 570 | 814 | 22 | 13.1 | 0.0006 | 0.75 | 1.30 | 5.26 | 1.73 |
| 74 | MLP & decision tree | 240 | 146 | 4 | 1.0 | 0.0001 | 2.02 | 1.60 | 5.26 | 4.18 |
| 75 | BERT & OpenAI | 506 | 70 | 4 | 1.0 | 0.0001 | 2.00 | 1.59 | 5.24 | 4.21 |
| 76 | NLTK & lemmatization | 570 | 447 | 14 | 7.2 | 0.0004 | 0.96 | 1.34 | 5.23 | 2.00 |
| 77 | RNN & embedding layer | 711 | 973 | 30 | 19.5 | 0.0008 | 0.62 | 1.25 | 5.10 | 1.58 |
| 78 | BoW & lexical features | 470 | 548 | 14 | 7.3 | 0.0004 | 0.95 | 1.32 | 5.07 | 1.98 |
| 79 | MLP & encoder | 240 | 573 | 9 | 3.9 | 0.0003 | 1.21 | 1.38 | 5.06 | 2.39 |
| 80 | embedding layer & pooling | 973 | 684 | 29 | 18.8 | 0.0008 | 0.63 | 1.24 | 5.03 | 1.59 |
| 81 | BiLSTM & RNN | 819 | 711 | 26 | 16.4 | 0.0007 | 0.66 | 1.24 | 4.97 | 1.62 |
| 82 | CoreNLP & POS tagging | 87 | 636 | 5 | 1.6 | 0.0001 | 1.68 | 1.46 | 4.92 | 3.35 |
| 83 | RNN & fully connected layer | 711 | 551 | 19 | 11.1 | 0.0005 | 0.78 | 1.26 | 4.90 | 1.76 |
| 84 | BoW __ feature selection | 470 | 204 | 7 | 2.7 | 0.0002 | 1.37 | 1.38 | 4.85 | 2.67 |
| 85 | classification __ rule based | 176 | 123 | 3 | 0.6 | 0.0001 | 2.30 | 1.61 | 4.85 | 5.08 |
| 86 | Bayes classifier __ KNN | 289 | 76 | 3 | 0.6 | 0.0001 | 2.27 | 1.60 | 4.80 | 5.04 |
| 87 | GBM __ decision tree | 150 | 146 | 3 | 0.6 | 0.0001 | 2.28 | 1.60 | 4.79 | 5.01 |
| 88 | PyTorch __ encoder | 169 | 573 | 7 | 2.7 | 0.0002 | 1.36 | 1.37 | 4.78 | 2.65 |
| 89 | BoW __ steeming | 470 | 352 | 10 | 4.7 | 0.0003 | 1.10 | 1.30 | 4.71 | 2.20 |
| 90 | ensemble model __ fully connected layers | 287 | 199 | 5 | 1.6 | 0.0001 | 1.63 | 1.42 | 4.64 | 3.19 |
| 91 | GBM __ bagging | 150 | 151 | 3 | 0.6 | 0.0001 | 2.23 | 1.56 | 4.63 | 4.84 |
| 92 | deleted punctuation __ lower case | 42 | 949 | 4 | 1.1 | 0.0001 | 1.83 | 1.44 | 4.61 | 3.84 |
| 93 | Scikit learn __ fully connected layers | 115 | 199 | 3 | 0.6 | 0.0001 | 2.22 | 1.55 | 4.58 | 4.80 |
| 94 | NER __ POS tagging | 227 | 636 | 9 | 4.1 | 0.0003 | 1.14 | 1.29 | 4.56 | 2.28 |
| 95 | POS tagging __ rule based | 636 | 123 | 6 | 2.2 | 0.0002 | 1.44 | 1.35 | 4.56 | 2.82 |

| | | | | | | | | | | |
|---|---|---|---|---|---|---|---|---|---|---|
| 96 | feature selection __ scikit-learn | 204 | 490 | 7 | 2.8 | 0.0002 | 1.31 | 1.31 | 4.49 | 2.56 |
| 97 | Bayes classifier __ feature selection | 289 | 204 | 5 | 1.7 | 0.0001 | 1.59 | 1.37 | 4.42 | 3.09 |
| 98 | lexical features __ linguistic features | 548 | 184 | 7 | 2.8 | 0.0002 | 1.30 | 1.30 | 4.42 | 2.54 |
| 99 | logistic regression __ scikit-learn | 771 | 490 | 18 | 10.7 | 0.0005 | 0.76 | 1.17 | 4.36 | 1.73 |
| 100 | RF __ decision tree | 412 | 146 | 5 | 1.7 | 0.0001 | 1.56 | 1.34 | 4.30 | 3.04 |

## 3. List of SemEval tasks (2012 – 2019)

Based on task description, we group each SemEval task within a task type. Then, due to a large number of task types, these were further clustered within 6 task groups:

- Sentiment Analysis (SA)
- Machine Translation (MT)
- Question Answering (QA)
- Information Extraction (IE) – information extraction, temporal information extraction, argument mining, fact checking
- Semantics Analysis (SEM) – semantic analysis, semantic difference, semantic inference, semantic role labeling, semantic parsing, semantic similarity, relational similarity
- Other (OT) – hypernym discovery, entity linking, lexical simplification, word sense disambiguation, taxonomy extraction, taxonomy enrichment

| Task ID | Full Name | Citations | Task Type | Task Group |
|---|---|---|---|---|
| 2012_01 | 1. English Lexical Simplification[1] | 103 | lexical simplification | OT |
| 2012_02 | 2. Measuring Degrees of Relational Similarity[2] | 122 | relational similarity | SEM |
| 2012_03 | 3. Spatial Role Labeling[3] | 39 | information extraction | IE |
| 2012_04 | 4. Evaluating Chinese Word Similarity[4] | 35 | semantic similarity | SEM |
| 2012_05 | 5. Chinese Semantic Dependency Parsing[5] | 16 | semantic parsing | SEM |
| 2012_06 | 6. Semantic Textual Similarity[6] | 363 | semantic similarity | SEM |
| 2012_07 | 7. COPA: Choice Of Plausible Alternatives An evaluation of commonsense causal reasoning[7] | 11 | question answering | QA |
| 2012_08 | 8. Cross-lingual Textual Entailment for Content Synchronization[8] | 34 | machine translation | MT |

---

[1] "SemEval-2012 Task 1: English Lexical Simplification - ACL ...." https://www.aclweb.org/anthology/S12-1046. Accessed 28 May. 2020.
[2] "SemEval-2012 Task 2: Measuring Degrees of Relational ...." 7 Jun. 2012, https://www.aclweb.org/anthology/S12-1047.pdf. Accessed 28 May. 2020.
[3] "SemEval-2013 Task 3: Spatial Role Labeling - ACL Anthology." https://www.aclweb.org/anthology/S13-2044. Accessed 28 May. 2020.
[4] "SemEval-2012 Task 4: Evaluating Chinese Word Similarity ...." https://www.aclweb.org/anthology/S12-1049. Accessed 28 May. 2020.
[5] "SemEval-2012 Task 5: Chinese Semantic Dependency Parsing." https://www.aclweb.org/anthology/S12-1050. Accessed 28 May. 2020.
[6] "SemEval-2012 Task 6: A Pilot on Semantic Textual Similarity ...." https://www.aclweb.org/anthology/S12-1051. Accessed 28 May. 2020.
[7] "SemEval-2012 Task 7: Choice of Plausible Alternatives: An ...." https://www.aclweb.org/anthology/S12-1052. Accessed 28 May. 2020.
[8] "Semeval-2012 Task 8: Cross-lingual Textual Entailment for ...." https://www.aclweb.org/anthology/S12-1053. Accessed 28 May. 2020.

| | | | | |
|---|---|---|---|---|
| 2013_01 | 1. TempEval-3 Temporal Annotation[9] | 213 | information extraction | IE |
| 2013_02 | 2. Sentiment Analysis in Twitter[10] | 195 | sentiment analysis | SA |
| 2013_03 | 3. Spatial Role Labeling[11] | 29 | information extraction | IE |
| 2013_04 | 4. Free Paraphrases of Noun Compounds[12] | 30 | semantic similarity | SEM |
| 2013_05 | 5. Evaluating Phrasal Semantics[13] | 23 | semantic inference | SEM |
| 2013_07 | 7. The Joint Student Response Analysis and 8th Recognizing Textual Entailment Challenge[14] | 76 | semantic inference | SEM |
| 2013_08 | 8. Cross-lingual Textual Entailment for Content Synchronization[15] | 10 | semantic inference | SEM |
| 2013_09 | 9. Extraction of Drug-Drug Interactions from BioMedical Texts[16] | 170 | information extraction | IE |
| 2013_10 | 10. Cross-lingual Word Sense Disambiguation[17] | 42 | machine translation | MT |
| 2013_11 | 11. Evaluating Word Sense Induction & Disambiguation within An End-User Application[18] | 48 | question answering | QA |
| 2013_12 | 12. Multilingual Word Sense Disambiguation[19] | 107 | semantic labeling | SEM |
| 2013_13 | 13. Word Sense Induction for Graded and Non-Graded Senses[20] | 49 | word sense disambiguation | OT |
| 2014_01 | 1. Evaluation of Compositional Distributional Semantic Models on Full Sentences through Semantic Relatedness and Entailment[21] | 374 | semantic similarity | SEM |
| 2014_02 | 2. Grammar Induction for Spoken Dialogue Systems[22] | 0 | semantic similarity | SEM |
| 2014_03 | 3. Cross-Level Semantic Similarity[23] | 42 | semantic similarity | SEM |
| 2014_04 | 4. Aspect Based Sentiment Analysis[24] | 344 | sentiment analysis | SA |

[9] "SemEval-2013 Task 1: TempEval-3: Evaluating Time ...." 14 Jun. 2013, https://www.aclweb.org/anthology/S13-2001.pdf. Accessed 28 May. 2020.
[10] "SemEval-2013 Task 2: Sentiment Analysis in Twitter." 14 Jun. 2013, https://www.aclweb.org/anthology/S13-2052.pdf. Accessed 28 May. 2020.
[11] "SemEval-2013 Task 3: Spatial Role Labeling - ACL Anthology." https://www.aclweb.org/anthology/S13-2044. Accessed 28 May. 2020.
[12] "SemEval-2013 Task 4: Free Paraphrases of Noun Compounds." https://www.aclweb.org/anthology/S13-2025. Accessed 28 May. 2020.
[13] "SemEval-2013 Task 5: Evaluating Phrasal Semantics - ACL ...." https://www.aclweb.org/anthology/S13-2007. Accessed 28 May. 2020.
[14] "SemEval-2013 Task 7: The Joint Student Response Analysis ...." https://www.aclweb.org/anthology/S13-2045. Accessed 28 May. 2020.
[15] "Semeval-2013 Task 8: Cross-lingual Textual Entailment ... - ACL." https://www.aclweb.org/anthology/S13-2005. Accessed 28 May. 2020.
[16] "SemEval-2013 Task 9 : Extraction of Drug-Drug Interactions ...." https://www.aclweb.org/anthology/S13-2056. Accessed 28 May. 2020.
[17] "SemEval-2013 Task 10: Cross-lingual Word Sense ... - cs.York." https://www.cs.york.ac.uk/semeval-2013/accepted/25_Paper.pdf. Accessed 28 May. 2020.
[18] "SemEval-2013 Task 11: Word Sense Induction and ...." https://www.aclweb.org/anthology/S13-2035. Accessed 28 May. 2020.
[19] "SemEval-2013 Task 12: Multilingual Word Sense ...." https://www.aclweb.org/anthology/S13-2040. Accessed 28 May. 2020.
[20] "SemEval-2013 Task 13: Word Sense Induction for Graded and ...." https://www.aclweb.org/anthology/S13-2049. Accessed 28 May. 2020.
[21] "SemEval-2014 Task 1: Evaluation of Compositional ...." 24 Aug. 2014, https://www.aclweb.org/anthology/S14-2001.pdf. Accessed 28 May. 2020.
[22] "Grammar Induction for Spoken Dialogue Systems - ACL ...." https://www.aclweb.org/anthology/S14-2002. Accessed 28 May. 2020.
[23] "SemEval-2014 Task 3: Cross-Level Semantic Similarity - ACL ...." https://www.aclweb.org/anthology/S14-2003. Accessed 28 May. 2020.
[24] "SemEval-2014 Task 4: Aspect Based Sentiment Analysis ...." https://www.aclweb.org/anthology/S14-2004. Accessed 28 May. 2020.

| | | | | |
|---|---|---|---|---|
| 2014_05 | 5. L2 Writing Assistant[25] | 4 | machine translation | MT |
| 2014_06 | 6. Supervised Semantic Parsing of Spatial Robot Commands[26] | 15 | semantic parsing | SEM |
| 2014_07 | 7. Analysis of Clinical Text[27] | 96 | information extraction | IE |
| 2014_08 | 8. Broad-Coverage Semantic Dependency Parsing[28] | 98 | semantic parsing | SEM |
| 2014_09 | 9. Sentiment Analysis in Twitter[29] | 3 | sentiment analysis | SA |
| 2014_10 | 10. Multilingual Semantic Textual Similarity[30] | 153 | semantic similarity | SEM |
| 2015_01 | Task 1: Paraphrase and Semantic Similarity in Tw[31]itter | 70 | semantic similarity | SEM |
| 2015_02 | Task 2: Semantic Textual Similarity, English, Spanish and Pilot on Interpretability[32] | 161 | semantic similarity | SEM |
| 2015_03 | Task 3: Answer Selection in Community Question Answering[33] | 56 | question answering | QA |
| 2015_04 | Task 4: TimeLine: Cross-Document Event Ordering[34] | 43 | temporal analysis | OT |
| 2015_05 | Task 5: QA TempEval[35] | 24 | temporal analysis | OT |
| 2015_06 | Task 6: Clinical TempEval[36] | 83 | information extraction | IE |
| 2015_07 | Task 7: Diachronic Text Evaluation[37] | 31 | information extraction | IE |
| 2015_08 | Task 8: SpaceEval[38] | 21 | information extraction | IE |
| 2015_09 | Task 9: CLIPEval Implicit Polarity of Events[39] | 13 | sentiment analysis | SA |
| 2015_10 | Task 10: Sentiment Analysis in Twitter[40] | 252 | sentiment analysis | SA |

[25] "SemEval 2014 Task 5 - L2 Writing Assistant - ACL Anthology." https://www.aclweb.org/anthology/S14-2005. Accessed 28 May. 2020.
[26] "SemEval-2014 Task 6: Supervised Semantic Parsing of ...." https://www.aclweb.org/anthology/S14-2006. Accessed 28 May. 2020.
[27] "SemEval-2014 Task 7: Analysis of Clinical Text - ACL Anthology." https://www.aclweb.org/anthology/S14-2007. Accessed 28 May. 2020.
[28] "SemEval 2014 Task 8: Broad-Coverage Semantic ... - ACL." https://www.aclweb.org/anthology/S14-2008. Accessed 28 May. 2020.
[29] "SemEval-2014 Task 9: Sentiment Analysis in Twitter - ACL." 24 Aug. 2014, https://www.aclweb.org/anthology/S14-2009.pdf. Accessed 28 May. 2020.
[30] "SemEval-2014 Task 10: Multilingual Semantic Textual Similarity." https://www.aclweb.org/anthology/S14-2010. Accessed 28 May. 2020.
[31] "SemEval-2015 Task 1: Paraphrase and Semantic Similarity in ...." https://www.aclweb.org/anthology/S15-2001. Accessed 28 May. 2020.
[32] "SemEval-2015 Task 2: Semantic Textual Similarity, English ...." https://www.aclweb.org/anthology/S15-2045. Accessed 28 May. 2020.
[33] "SemEval-2015 Task 3: Answer Selection in Community ...." https://www.aclweb.org/anthology/S15-2047. Accessed 28 May. 2020.
[34] "SemEval-2015 Task 4: TimeLine: Cross-Document Event ...." https://www.aclweb.org/anthology/S15-2132. Accessed 28 May. 2020.
[35] "SemEval-2015 Task 5: QA TempEval - Evaluating Temporal ...." https://www.aclweb.org/anthology/S15-2134. Accessed 28 May. 2020.
[36] "SemEval-2015 Task 6: Clinical TempEval - ACL Anthology." https://www.aclweb.org/anthology/S15-2136. Accessed 28 May. 2020.
[37] "SemEval 2015, Task 7: Diachronic Text Evaluation." https://www.aclweb.org/anthology/S15-2147.pdf. Accessed 28 May. 2020.
[38] "SemEval-2015 Task 8: SpaceEval - ACL Anthology." https://www.aclweb.org/anthology/S15-2149. Accessed 28 May. 2020.
[39] "SemEval-2015 Task 9: CLIPEval Implicit Polarity of Events ...." https://www.aclweb.org/anthology/S15-2077. Accessed 28 May. 2020.
[40] "SemEval-2015 Task 10: Sentiment Analysis in Twitter - ACL ...." https://www.aclweb.org/anthology/S15-2078. Accessed 28 May. 2020.

| | | | | |
|---|---|---|---|---|
| 2015_11 | Task 11: Sentiment Analysis of Figurative Language in Twitter[41] | 102 | sentiment analysis | SA |
| 2015_12 | Task 12: Aspect Based Sentiment Analysis[42] | 214 | sentiment analysis | SA |
| 2015_13 | Task 13: Multilingual All-Words Sense Disambiguation and Entity Linking[43] | 85 | entity linking | OT |
| 2015_14 | Task 14: Analysis of Clinical Text[44] | 53 | information extraction | IE |
| 2015_15 | Task 15: A CPA Dictionary-Entry-Building Task[45] | 2 | semantic parsing | SEM |
| 2015_17 | Task 17: Taxonomy Extraction Evaluation[46] | 43 | taxonomy extraction | OT |
| 2015_18 | Task 18: Semantic Dependency Parsing[47] | 0 | semantic parsing | SEM |
| 2016_01 | Task 1: Semantic Textual Similarity, Monolingual and Cross-Lingual Evaluation[48] | 150 | semantic similarity | SEM |
| 2016_02 | Task 2: Interpretable Semantic Textual Similarity[49] | 26 | semantic similarity | SEM |
| 2016_03 | Task 3: Community Question Answering[50] | 123 | semantic similarity | SEM |
| 2016_04 | Task 4: Sentiment Analysis in Twitter[51] | 436 | sentiment analysis | SA |
| 2016_05 | Task 5: Aspect-Based Sentiment Analysis[52] | 465 | sentiment analysis | SA |
| 2016_06 | Task 6: Detecting Stance in Tweets[53] | 209 | sentiment analysis | SA |
| 2016_07 | Task 7: Determining Sentiment Intensity of English and Arabic Phrases[54] | 39 | sentiment analysis | SA |
| 2016_08 | Task 8: Meaning Representation Parsing[55] | 28 | semantic parsing | SEM |
| 2016_09 | Task 9: Chinese Semantic Dependency Parsing[56] | 0 | semantic parsing | SEM |

[41] "SemEval-2015 Task 11: Sentiment Analysis of Figurative ...." http://alt.qcri.org/semeval2015/task11/. Accessed 28 May. 2020.
[42] "SemEval-2015 Task 12: Aspect Based Sentiment Analysis ...." https://www.aclweb.org/anthology/S15-2082/. Accessed 28 May. 2020.
[43] "SemEval-2015 Task 13: Multilingual All-Words Sense ... - ACL." https://www.aclweb.org/anthology/S15-2049. Accessed 28 May. 2020.
[44] "SemEval-2015 Task 14: Analysis of Clinical Text - ACL ...." https://www.aclweb.org/anthology/S15-2051. Accessed 28 May. 2020.
[45] "SemEval-2015 Task 15: A CPA dictionary-entry-building task." https://www.aclweb.org/anthology/S15-2053.pdf. Accessed 28 May. 2020.
[46] "SemEval-2015 Task 17: Taxonomy Extraction Evaluation ...." https://www.aclweb.org/anthology/S15-2151. Accessed 28 May. 2020.
[47] "SemEval 2015 Task 18: Broad-Coverage Semantic ...." https://www.aclweb.org/anthology/S15-2153. Accessed 28 May. 2020.
[48] "SemEval-2016 Task 1: Semantic Textual Similarity ...." https://www.aclweb.org/anthology/S16-1081. Accessed 28 May. 2020.
[49] "SemEval-2016 Task 2: Interpretable Semantic Textual Similarity." https://www.aclweb.org/anthology/S16-1082. Accessed 28 May. 2020.
[50] "SemEval-2016 Task 3: Community Question Answering - ACL ...." https://www.aclweb.org/anthology/S16-1083. Accessed 28 May. 2020.
[51] "SemEval-2016 Task 4: Sentiment Analysis in Twitter - ACL ...." https://www.aclweb.org/anthology/S16-1001. Accessed 28 May. 2020.
[52] "SemEval-2016 Task 5: Aspect Based Sentiment Analysis ...." https://www.aclweb.org/anthology/S16-1002. Accessed 28 May. 2020.
[53] "SemEval-2016 Task 6: Detecting Stance in Tweets - ACL ...." https://www.aclweb.org/anthology/S16-1003. Accessed 28 May. 2020.
[54] "SemEval-2016 Task 7: Determining Sentiment Intensity ... - ACL." https://www.aclweb.org/anthology/S16-1004. Accessed 28 May. 2020.
[55] "SemEval-2016 Task 8: Meaning Representation Parsing ...." https://www.aclweb.org/anthology/S16-1166. Accessed 28 May. 2020.
[56] "SemEval-2016 Task 9: Chinese Semantic Dependency Parsing." https://www.aclweb.org/anthology/S16-1167. Accessed 28 May. 2020.

| | | | | |
|---|---|---|---|---|
| 2016_10 | Task 10: Detecting Minimal Semantic Units and their Meanings[57] | 23 | semantic analysis | SEM |
| 2016_11 | Task 11: Complex Word Identification[58] | 40 | lexical simplification | OT |
| 2016_12 | Task 12: Clinical TempEval[59] | 79 | information extraction | IE |
| 2016_13 | Task 13: Taxonomy Extraction Evaluation (TExEval-2)[60] | 54 | taxonomy extraction | OT |
| 2016_14 | Task 14: Semantic Taxonomy Enrichment[61] | 10 | taxonomy enrichment | OT |
| 2017_01 | Task 1: Semantic Textual Similarity[62] | 144 | semantic similarity | SEM |
| 2017_02 | Task 2: Multi-lingual and Cross-lingual Semantic Word Similarity[63] | 56 | semantic similarity | SEM |
| 2017_03 | Task 3: Community Question Answering[64] | 106 | semantic similarity | SEM |
| 2017_04 | Task 4: Sentiment Analysis in Twitter[65] | 307 | sentiment analysis | SA |
| 2017_05 | Task 5: Fine-Grained Sentiment Analysis on Financial Microblogs and News[66] | 48 | sentiment analysis | SA |
| 2017_06 | Task 6: #HashtagWars: Learning a Sense of Humor[67] | 15 | sentiment analysis | SA |
| 2017_07 | Task 7: Detection and Interpretation of English Puns[68] | 23 | semantic parsing | SEM |
| 2017_08 | Task 8: RumourEval: Determining rumour veracity and support for rumours[69] | 71 | fact checking | IE |
| 2017_09 | Task 9: Abstract Meaning Representation Parsing and Generation[70] | 15 | semantic parsing | SEM |
| 2017_10 | Task 10: Extracting Keyphrases and Relations from Scientific Publications[71] | 73 | information extraction | IE |
| 2017_11 | Task 11: End-User Development using Natural Language[72] | 4 | machine translation | MT |

[57] "SemEval-2016 Task 10: Detecting Minimal Semantic Units ...." https://www.aclweb.org/anthology/S16-1084. Accessed 28 May. 2020.
[58] "SemEval 2016 Task 11: Complex Word Identification - ACL ...." https://www.aclweb.org/anthology/S16-1085. Accessed 28 May. 2020.
[59] "SemEval-2017 Task 12: Clinical TempEval - ACL Anthology." https://www.aclweb.org/anthology/S17-2093. Accessed 28 May. 2020.
[60] "SemEval-2016 Task 13: Taxonomy Extraction Evaluation ...." https://www.aclweb.org/anthology/S16-1168. Accessed 28 May. 2020.
[61] "SemEval-2016 Task 14: Semantic Taxonomy Enrichment ...." https://www.aclweb.org/anthology/S16-1169. Accessed 28 May. 2020.
[62] "SemEval-2017 Task 1: Semantic Textual Similarity ...." https://www.aclweb.org/anthology/S17-2001. Accessed 28 May. 2020.
[63] "SemEval-2017 Task 2: Multilingual and Cross-lingual Semantic." https://www.aclweb.org/anthology/S17-2002. Accessed 28 May. 2020.
[64] "SemEval-2016 Task 3: Community Question Answering - ACL ...." https://www.aclweb.org/anthology/S16-1083. Accessed 28 May. 2020.
[65] "SemEval-2016 Task 4: Sentiment Analysis in Twitter - ACL ...." https://www.aclweb.org/anthology/S16-1001. Accessed 28 May. 2020.
[66] "SemEval-2017 Task 5: Fine-Grained Sentiment Analysis on ...." https://www.aclweb.org/anthology/S17-2089/. Accessed 28 May. 2020.
[67] "SemEval-2017 Task 6: #HashtagWars: Learning a Sense of ...." https://www.aclweb.org/anthology/S17-2004. Accessed 28 May. 2020.
[68] "SemEval-2017 Task 7: Detection and Interpretation of English ...." https://www.aclweb.org/anthology/S17-2005. Accessed 28 May. 2020.
[69] "SemEval-2017 Task 8: RumourEval: Determining rumour ...." https://www.aclweb.org/anthology/S17-2006. Accessed 28 May. 2020.
[70] "SemEval-2017 Task 9: Abstract Meaning Representation ...." https://www.aclweb.org/anthology/S17-2090. Accessed 28 May. 2020.
[71] "SemEval 2017 Task 10: ScienceIE - Extracting Keyphrases ...." https://www.aclweb.org/anthology/S17-2091. Accessed 28 May. 2020.
[72] "End-User Development using Natural Language - ACL ...." https://www.aclweb.org/anthology/S17-2092. Accessed 28 May. 2020.

| | | | | |
|---|---|---|---|---|
| 2017_12 | Task 12: Clinical TempEval[73] | 0 | information extraction | IE |
| 2018_01 | Task 1: Affect in Tweets[74] | 98 | sentiment analysis | SA |
| 2018_02 | Task 2: Multilingual Emoji Prediction[75] | 20 | sentiment analysis | SA |
| 2018_03 | Task 3: Irony Detection in English Tweets[76] | 43 | sentiment analysis | SA |
| 2018_04 | Task 4: Character Identification on Multiparty Dialogues[77] | 2 | entity linking | OT |
| 2018_05 | Task 5: Counting Events and Participants within Highly Ambiguous Data covering a very long tail[78] | 0 | question answering | QA |
| 2018_06 | Task 6: Parsing Time Normalizations[79] | 3 | information extraction | IE |
| 2018_07 | Task 7: Semantic Relation Extraction and Classification in Scientific Papers[80] | 26 | semantic parsing | SEM |
| 2018_08 | Task 8: Semantic Extraction from CybersecUrity REports using Natural Language Processing (SecureNLP)[81] | 3 | information extraction | IE |
| 2018_09 | Task 9: Hypernym Discovery[82] | 13 | hypernym discovery | OT |
| 2018_10 | Task 10: Capturing Discriminative Attributes[83] | 5 | semantic difference | SEM |
| 2018_11 | Task 11: Machine Comprehension using Commonsense Knowledge[84] | 33 | question answering | QA |
| 2018_12 | Task 12: Argument Reasoning Comprehension Task[85] | 7 | argument reasoning | IE |
| 2019_01 | Task 1: Cross-lingual Semantic Parsing with UCCA[86] | 3 | semantic parsing | SEM |
| 2019_02 | Task 2: Unsupervised Lexical Semantic Frame Induction[87] | 1 | semantic labeling | SEM |
| 2019_03 | Task 3: EmoContext: Contextual Emotion Detection in Text[88] | 11 | sentiment analysis | SA |

73 "SemEval-2017 Task 12: Clinical TempEval - ACL Anthology." https://www.aclweb.org/anthology/S17-2093. Accessed 28 May. 2020.
74 "SemEval-2018 Task 1: Affect in Tweets - ACL Anthology." https://www.aclweb.org/anthology/S18-1001. Accessed 28 May. 2020.
75 "SemEval 2018 Task 2: Multilingual Emoji Prediction - ACL ...." https://www.aclweb.org/anthology/S18-1003. Accessed 28 May. 2020.
76 "SemEval-2018 Task 3: Irony Detection in English Tweets ...." https://www.aclweb.org/anthology/S18-1005. Accessed 28 May. 2020.
77 "SemEval 2018 Task 4: Character Identification on Multiparty ...." https://www.aclweb.org/anthology/S18-1007. Accessed 28 May. 2020.
78 "SemEval-2018 Task 5: Counting Events and Participants in ...." 5 Jun. 2018, https://www.aclweb.org/anthology/S18-1009.pdf. Accessed 28 May. 2020.
79 "SemEval 2018 Task 6: Parsing Time Normalizations - ACL ...." https://www.aclweb.org/anthology/S18-1011. Accessed 28 May. 2020.
80 "SemEval-2018 Task 7: Semantic Relation Extraction and ...." https://www.aclweb.org/anthology/S18-1111. Accessed 28 May. 2020.
81 "SemEval-2018 Task 8: Semantic Extraction from ... - ACL." https://www.aclweb.org/anthology/S18-1113. Accessed 28 May. 2020.
82 "SemEval-2018 Task 9: Hypernym Discovery - ACL Anthology." https://www.aclweb.org/anthology/S18-1115. Accessed 28 May. 2020.
83 "SemEval-2018 Task 10: Capturing Discriminative Attributes ...." https://www.aclweb.org/anthology/S18-1117. Accessed 28 May. 2020.
84 "SemEval-2018 Task 11: Machine Comprehension Using - ACL." https://www.aclweb.org/anthology/S18-1119. Accessed 28 May. 2020.
85 "SemEval-2018 Task 12: The Argument Reasoning ... - ACL." https://www.aclweb.org/anthology/S18-1121. Accessed 28 May. 2020.
86 "SemEval-2019 Task 1: Cross-lingual Semantic Parsing with ...." https://www.aclweb.org/anthology/S19-2001. Accessed 28 May. 2020.
87 "SemEval-2019 Task 2: Unsupervised Lexical Frame Induction ...." https://www.aclweb.org/anthology/S19-2003. Accessed 28 May. 2020.
88 "SemEval-2019 Task 3: EmoContext Contextual Emotion ...." https://www.aclweb.org/anthology/S19-2005. Accessed 28 May. 2020.

| | | | | |
|---|---|---|---|---|
| 2019_04 | Task 4: Hyperpartisan News Detection[89] | 5 | sentiment analysis | SA |
| 2019_05 | Task 5: HatEval: Multilingual Detection of Hate Speech Against Immigrants and Women in Twitter[90] | 15 | sentiment analysis | SA |
| 2019_06 | Task 6: OffensEval: Identifying and Categorizing Offensive Language in Social Media[91] | 13 | sentiment analysis | SA |
| 2019_07 | Task 7: RumourEval 2019: Determining Rumour Veracity and Support for Rumours[92] | 7 | fact checking | IE |
| 2019_08 | Task 8: Fact Checking in Community Question Answering Forums[93] | 4 | fact checking | IE |
| 2019_09 | Task 9: Suggestion Mining from Online Reviews and Forums[94] | 3 | information extraction | IE |
| 2019_10 | Task 10: Math Question Answering[95] | 0 | question answering | QA |
| 2019_12 | Task 12: Toponym Resolution in Scientific Papers[96] | 2 | entity linking | OT |

89 "SemEval-2019 Task 4: Hyperpartisan News Detection - ACL ...." https://www.aclweb.org/anthology/S19-2145. Accessed 28 May. 2020.
90 "SemEval-2019 Task 5: Multilingual Detection of Hate Speech ...." https://www.aclweb.org/anthology/S19-2007. Accessed 3 Jun. 2020.
91 "SemEval-2019 Task 6: Identifying and Categorizing Offensive ...." https://www.aclweb.org/anthology/S19-2010. Accessed 28 May. 2020.
92 "SemEval-2019 Task 7: RumourEval, Determining Rumour ...." https://www.aclweb.org/anthology/S19-2147. Accessed 28 May. 2020.
93 "SemEval-2019 Task 8: Fact Checking in Community Question ...." https://www.aclweb.org/anthology/S19-2149. Accessed 28 May. 2020.
94 "SemEval-2019 Task 9: Suggestion Mining from Online ...." https://www.aclweb.org/anthology/S19-2151. Accessed 28 May. 2020.
95 "SemEval-2019 Task 10: Math Question Answering - ACL ...." https://www.aclweb.org/anthology/S19-2153. Accessed 28 May. 2020.
96 "SemEval-2019 Task 12: Toponym Resolution in Scientific ...." https://www.aclweb.org/anthology/S19-2155. Accessed 28 May. 2020.
